# Supplementary material for: Scaling Optimization Over Uncertainty via Compilation
Source: arXiv:2502.18728 source file (2025-04-10)
Supplement: Supplementary file 1 [file additional-problems.tex]

\subsection{An additional problem for BBIR representation}\label{subsec:sensitivity}

The \textit{sensitivity} of a probabilistic program  
measures the degree to which the inputs to a program may affect the output.
A main application is in algorithmic stability, in 
which we want to diagnose which configurations of an algorithm are most stable 
under varying input~\citep{aguirre2021pre}.
This sensitivity is often computed by bounding a notion of distance between two
possible distributions, such as the total variation distance:

\begin{definition}[Total variation distance~\citep{levin2017markov}]
  The total variation (TV) distance between two distributions 
  $\mu_1, \mu_2$ over the same finite set of random variables $X$
  is $TV(\mu_1, \mu_2) \triangleq \sum_{x \in X} \frac{|\mu_1(x)-\mu_2(x)|}{2}$. 
\end{definition}

In the case of a Boolean formula $\varphi$
% and a weight function
% $w : lits(\varphi) \to [0,1]$, it is known
% that $\AMC(\varphi, w)$ 
the AMC can
specify a distribution on the models of $\varphi$ with an appropriate weight 
function~\citep{de2007problog,holtzen2020scaling}. With this in mind, 
we can consider a discrete probabilistic program 
with a set
$I$ of Boolean inputs. The output of this program will be a 
distribution over models of the program satisfying the input. 

\citet{aguirre2021pre} consider the problem of bounding the expected
sensitivity of a probabilistic program.  In this setting it is 
also interesting to ask: what is the \textit{maximum}
sensitivity of a probabilistic program? This problem can be captured 
by the following BBIR where $(\{\varphi\}, I, w)$

\begin{enumerate}[leftmargin=*]
  \item $\varphi$ is the compiled probabilistic program as a Boolean formula,
  following existing strategies in the literature~\citep{holtzen2020scaling,de2007problog,saad2021sppl},
  \item $I$ the input variables,
  \item $w$ the weight function with codomain in the real branch-and-bound semiring
  $\R$ as per the previous example.
\end{enumerate}

Then the maximum probabilistic sensitivity problem will be:
\begin{equation}
  \begin{split}
  \mathrm{Sens}{(\{\varphi\}, I, w)} 
  &= \max_{(i,j) \in inst(I) \times inst(I)} TV(\varphi|_i, \varphi|_j).
  % & = \max_{(i,j) \in inst(I) \times inst(I)} \sum_{m \models \varphi|_i \lor \varphi|_j}
  %   \frac{|\Pr[\{m \models \varphi|_i\}] -\Pr[\{m \models \varphi|_j\}]|}{2}
\end{split}
\end{equation}
